# Supplementary material for: End-to-End Video Captioning
Source: arXiv:1904.02628 source file (2019-11-08)
Supplement: Supplementary file 1 [file suppmat.tex]

%\section{Supplementary Material}

We show the additional materials about our work. 
In particular, we are going to add more qualitative results of our models, 
focusing on the difference between the two steps. Specifically, we analyse: (i) when step 2 improves over step 1; (ii) when step 2 does not improve the step 1;  (iii) negative samples, i.e. when both the steps produce wrong captions.

The improvement of the model from step 1 to step 2 that we have found are summarised in the  Tables \ref{tab:S2BestMSVDGLN}, \ref{tab:S2BestMSVDIRv2} and \ref{tab:S2BestMSR-VTT}.  As we expected, fine-tuning the model allows correcting the wrong words in the caption without changes the entire sentence (rows 1, 5 Table \ref{tab:S2BestMSVDGLN}; rows 1, 2 Table \ref{tab:S2BestMSR-VTT}). Also, it can add new information about the action, e.g. new words in the sentence (rows 5, 7, 8 in Table \ref{tab:S2BestMSR-VTT}). 
Although, the second step improves most of the example of the test set, but, some of them show the opposite results. On the MSVD dataset (Table \ref{tab:S1BestMSVD}) it recurs in few elements, while in the MSR-VTT the model wrong to predict the subject or object of the action (rows 5, 7 in Table \ref{tab:S1BestMSR-VTT}). 
Some negative example are showed in table \ref{tab:NegExampleMSVD} and \ref{tab:NegExampleMSR-VTT}. Many rows like 1, 2, 5, 6 in Table \ref{tab:NegExampleMSVD} and 1, 2, 3, 4 in Table \ref{tab:NegExampleMSR-VTT} shows how to try the improvements of the model (step 2) in such cases does not work, in fact, the prediction does not change. On the other case (rows 10 in Table \ref{tab:NegExampleMSVD} and rows 5, 8 in Table \ref{tab:NegExampleMSR-VTT}) the changes just lead to mistakes in a different way. 
Finally, MSVD dataset allows to create a model that predicts a simple sentence, while the model trained using the MSR-VTT one creates longer sentences. Our framework is, therefore, able to provide reasonable predictions in both cases.

\newpage
% The step 2 does not improve the step 1 - MSVD - EtENet-GLN & EtENet-IRv2
\begin{table}[h!]
\begin{center}
\begin{tabular}{|l|p{6cm}|}
\hline
\multicolumn{2}{|c|}{EtENet-GLN} \\
\hline
Step 1 & \bf{a man is eating something} \\
Step 2 & {a man is eating a flute} \\
References & \emph{a man eats spaghetti}; 
\emph{a man is eating something}; 
\emph{a person is eating}; \\
\hline
Step 1 & \bf{two women are dancing} \\
Step 2 & {two men are fighting} \\
References & \emph{a group of people are dancing}; 
\emph{several people are dancing on the patio}; 
\emph{some people are dancing}; \\
\hline
Step 1 & \bf{a baby is eating} \\
Step 2 & {a baby is talking} \\
References & \emph{a baby is eating ice cream}; 
\emph{a child is laughing}; 
\emph{a baby holding ice cream is laughing}; \\
\hline
Step 1 & \bf{a man is playing a piano} \\
Step 2 & {a man is playing a guitar} \\
References & \emph{a man is playing a keyboard piano}; 
\emph{a man is playing an electric keyboard}; 
\emph{a man plays on the electronic musical instrument}; \\
\hline
%Step 1 & \bf{two men are fighting} \\
%Step 2 & {a man is talking} \\
%References & \emph{two men appear to be fighting or wrestling}; 
%\emph{two men are fighting}; 
%\emph{a man is fighting with the other man}; \\
%\hline
\multicolumn{2}{|c|}{EtENet-IRv2} \\
\hline
Step 1 & \bf{men are playing basketball} \\
Step 2 & {men are playing soccer} \\
References & \emph{a basketball game is in play}; 
\emph{two teams are playing basketball on television}; 
\emph{men are playing basketball}; \\
\hline
Step 1 & \bf{two men are fighting} \\
Step 2 & {a man is talking} \\
References & \emph{two men are fighting};
\emph{two men are fighting with each other};
\emph{two men appear to be fighting or wrestling}; \\
\hline
%Step 1 & \bf{a man is climbing on a rope} \\
%Step 2 & {a man is jumping on a rope} \\
%References & \emph{a man and boy are rock climbing};
%\emph{a boy is rock climbing};
%\emph{the girl is climing the rock wall}; \\
%\hline
Step 1 & \bf{a man is playing cricket} \\
Step 2 & {a man is playing football} \\
References & \emph{two teams are playing cricket};
\emph{people are playing cricket};
\emph{a man in cricket performs an error}; \\
\hline
\end{tabular}
\end{center}
\caption{Some qualitative examples in which the step 2 does not improve over the step 1 on the MSVD dataset. Bold text means the best results.}
\label{tab:S1BestMSVD}
\end{table}

\clearpage
\newpage
% The step 2 does not improve the step 1 - MSR-VTT 
\begin{table}[h!]
\begin{center}
\begin{tabular}{|l|p{6cm}|}
\hline
\multicolumn{2}{|c|}{EtENet-IRv2} \\
\hline
Step 1 & \bf{a man is playing a baseball game} \\
Step 2 & {a man is running on a field} \\
References & \emph{a baseball game is played}; 
\emph{players hitting baseballs with bat}; 
\emph{a man is hitting the ball in a baseball game}; \\
\hline
Step 1 & \bf{a group of people are dancing} \\
Step 2 & {a group of people are walking down the street} \\
References & \emph{a dance class where people are learning footwork};
\emph{a large class of men and woman taking dance lessons in a studio};
\emph{a ballroom dance class}; \\
\hline
Step 1 & \bf{a person is mixing ingredients in a bowl} \\
Step 2 & {a woman is mixing ingredients in a bowl} \\
References & \emph{a woman mixes batter in a bowl};
\emph{a chef stirs flower with water};
\emph{a woman is saying how to make nabeyaki udon noodle}; \\
\hline
Step 1 & \bf{there is a fish swimming in the water} \\
Step 2 & {a fish swimming in a swimming pool} \\
References & \emph{two orange and white fish are swimming together};
\emph{there are two fish floating in to the water};
\emph{a fish tank with two gold fish and plants}; \\
\hline
Step 1 & \bf{a baby is walking} \\
Step 2 & {a turtle is walking} \\
References & \emph{a turtle is walking underwater};
\emph{a turtle is swimming in water};
\emph{the turtle is moving under water}; \\
\hline
Step 1 & \bf{a man is talking to a crowd of people} \\
Step 2 & {a group of people are walking on a stage} \\
References & \emph{a man calls out a young girl s name to walk onto the stage};
\emph{a man is singing to a crowd};
\emph{annual day celebrations are going on}; \\
\hline
Step 1 & \bf{a group of people are playing basketball} \\
Step 2 & {a man is running on a trampoline} \\
References & \emph{a group of young people play basketball together outside};
\emph{people playing basketball and also performing trick shots and bloopers};
\emph{a basketball player swats a ball when it is shot}; \\
\hline
Step 1 & \bf{a man is talking about a car} \\
Step 2 & {a man is explaining something} \\
References & \emph{a demonstration of a broken part to a vehicle};
\emph{a guy talking about car parts};
\emph{a man is repairing a car}; \\
\hline
\end{tabular}
\end{center}
\caption{Some qualitative examples with EtENet-IRv2 model in which the step 2 does not improve the step 1 using 
the MSR-VTT dataset. Bold text means the best results.}
\label{tab:S1BestMSR-VTT}
\end{table}

\newpage
% The step 2 improve the step 1 - MSVD - EtENet-GLN
\begin{table}[h!]
\begin{center}
\begin{tabular}{|l|p{6cm}|}
\hline
\multicolumn{2}{|c|}{EtENet-GLN} \\
\hline
Step 1 & {a man is dancing} \\
Step 2 & \bf{a woman is dancing} \\
References & \emph{a girl is dancing}; 
\emph{a woman does aerobic exercise}; 
\emph{a woman is exercising}; \\
\hline
Step 1 & {a polar bear is floating on the water} \\
Step 2 & \bf{a polar bear is walking} \\
References & \emph{a polar bear is running toward walruses};
\emph{a polar bear is walking};
\emph{bears are running}; \\
\hline
Step 1 & {a man is cooking} \\
Step 2 & \bf{a man is pouring sauce in a pot} \\
References & \emph{a man is pouring wine into a pot};
\emph{a person is adding souse in the pot};
\emph{a person making spaghetti sauce}; \\
\hline
Step 1 & {a group of men are dancing} \\
Step 2 & \bf{a man is dancing} \\
References & \emph{a man is dancing};
\emph{a man is dancing on stage};
\emph{a person is dancing}; \\
\hline
Step 1 & {a woman is slicing a carrot} \\
Step 2 & \bf{a woman is slicing a tomato} \\
References & \emph{a person is slicing a tomato};
\emph{a woman is slicing tomato};
\emph{a chef is slicing a tomato}; \\
\hline
Step 1 & {a dog is walking} \\
Step 2 & \bf{a panda is playing} \\
References & \emph{a baby panda is going down a slide};
\emph{pandas are playing};
\emph{panda babies are playing}; \\
\hline
Step 1 & {a man is pouring sauce into a bowl} \\
Step 2 & \bf{a woman is adding water into a bowl} \\
References & \emph{someone is pouring water into a plastic bowl of mushrooms};
\emph{a woman pours some water on an unknown brown food};
\emph{a woman is mixing ingredients}; \\
\hline
Step 1 & {a man is dancing} \\
Step 2 & \bf{a man is riding a motorcycle} \\
References & \emph{a man and woman ride a motorcycle};
\emph{a lovers is riding on the motor bike};
\emph{a man and woman are driving on a motorcycle}; \\
\hline
Step 1 & {a band is singing} \\
Step 2 & \bf{a woman is singing} \\
References & \emph{a woman is singing into a hand-held microphone on stage};
\emph{a woman is singing};
\emph{a girl is singing on stage}; \\
\hline
\end{tabular}
\end{center}
\caption{Some qualitative examples with EtENet-GLN model in which the step 2 improve the step 1 using the MSVD dataset. Bold text means the best results.}
\label{tab:S2BestMSVDGLN}
\end{table}

\newpage
% The step 2 improve the step 1 - MSVD - EtENet-IRv2
\begin{table}[h!]
\begin{center}
\begin{tabular}{|l|p{6cm}|}
\hline
\multicolumn{2}{|c|}{EtENet-IRv2} \\
\hline
Step 1 & {a woman is slicing some bread} \\
Step 2 & \bf{a woman is slicing a potato} \\
References & \emph{a woman is piercing potato}; 
\emph{a lady is cooking food}; 
\emph{a woman is stabbing a potato with a fork}; \\
\hline
Step 1 & {a man is reading} \\
Step 2 & \bf{a man is talking} \\
References & \emph{a man is talking};
\emph{a man talks};
\emph{a man is speaking directly to the camera}; \\
\hline
Step 1 & {a person is mixing ingredients in a bowl} \\
Step 2 & \bf{a woman is mixing ingredients in a bowl} \\
References & \emph{a woman mixes batter in a bowl};
\emph{a chef stirs flower with water};
\emph{a woman is saying how to make nabeyaki udon noodle}; \\
\hline
Step 1 & {a woman is slicing a cucumber} \\
Step 2 & \bf{a woman is slicing an onion} \\
References & \emph{a woman is slicing an onion};
\emph{a woman cuts onion};
\emph{a woman slices onions with a large knife}; \\
\hline
Step 1 & {a baby is walking} \\
Step 2 & \bf{a turtle is walking} \\
References & \emph{a turtle is walking underwater};
\emph{a turtle is swimming in water};
\emph{the turtle is moving under water}; \\
\hline
Step 1 & {a woman is drawing a piece of paper} \\
Step 2 & \bf{a woman is cutting a piece of paper} \\
References & \emph{a person is cutting a piece of paper};
\emph{a woman is cutting papers};
\emph{a woman is cutting a paper with a scissors}; \\
\hline
Step 1 & {a man is playing with a man} \\
Step 2 & \bf{a man is playing a guitar} \\
References & \emph{a man is playing the guitar};
\emph{a man is sitting and playing a small guitar};
\emph{the homeless guy played his ukelele on the street}; \\
\hline
Step 1 & {a man and a woman are dancing} \\
Step 2 & \bf{a man is riding a boat} \\
References & \emph{the woman is paddling a canoe};
\emph{a woman is rowing a boat};
\emph{a lady is rowing a boat}; \\
\hline
Step 1 & {a person is cooking} \\
Step 2 & \bf{a person is cutting meat} \\
References & \emph{a person is chopping meat};
\emph{the person is slicing meat};
\emph{a man is chopping beef using a large flat kitchen knife}; \\
\hline
\end{tabular}
\end{center}
\caption{Some qualitative examples with EtENet-IRv2 model in which the step 2 improve the step 1 using the MSVD dataset. Bold text means the best results.}
\label{tab:S2BestMSVDIRv2}
\end{table}

\newpage
% The step 2 improve the step 1 - MSR-VTT
\begin{table}[t!]
\begin{center}
\begin{tabular}{|l|p{6cm}|}
\hline
\multicolumn{2}{|c|}{EtENet-IRv2} \\
\hline
Step 1 & {a person is playing a football game} \\
Step 2 & \bf{a man is talking about football} \\
References & \emph{a man is talking about a sports match};
\emph{guy speaking about matt ryan s new contract};
\emph{a man talks about matt ryan while still frames are shown}; \\
\hline
Step 1 & {a person is playing with toys} \\
Step 2 & \bf{a man is playing with a dog} \\
References & \emph{a couple talk about their dog};
\emph{a couple is shown with many pictures of their dog};
\emph{people are talking and holding a dog}; \\
\hline
Step 1 & {a person is mixing ingredients in a bowl} \\
Step 2 & \bf{a woman is mixing ingredients in a bowl} \\
References & \emph{a woman mixes batter in a bowl};
\emph{a chef stirs flower with water};
\emph{a woman is saying how to make nabeyaki udon noodle}; \\
\hline
Step 1 & {a man is talking} \\
Step 2 & \bf{a man is talking to another man} \\
References & \emph{a man is talking to another man};
\emph{a man talking to another guy};
\emph{two men are talking in a dark room}; \\
\hline
Step 1 & {a man is riding a boat in the ocean} \\
Step 2 & \bf{a man in a blue shirt is swimming in the ocean} \\
References & \emph{there is a man in blue is swimming in the sea};
\emph{there is a man in blue is talking nearby the beach};
\emph{a man in blue shirt swims with big waves then gets on back of a jet ski}; \\
\hline
Step 1 & {a woman is talking to a woman} \\
Step 2 & \bf{a woman is cooking food} \\
References & \emph{man and woman on cooking show};
\emph{a man stirs a bowl of mashed potatoes};
\emph{a chef is making a dough}; \\
\hline
Step 1 & {two men are playing table tennis} \\
Step 2 & \bf{a man in a blue shirt is talking about ping pong} \\
References & \emph{a man describes a good ping pong stroke including keeping the paddle about head high};
\emph{ping pong player explaining about some tricks to win matches};
\emph{a left hand blue tshirt person is play table tennis}; \\
\hline
Step 1 & {a man is singing} \\
Step 2 & \bf{a man and a woman are talking to each other} \\
References & \emph{a man and a woman are having a conversation};
\emph{woman is talking with man};
\emph{woman talks about poetry and love}; \\
\hline
\end{tabular}
\end{center}
\caption{Some qualitative examples with EtENet-IRv2 model in which the step 2 improve the step 1 using the MSR-VTT dataset. Bold text means the best results.}
\label{tab:S2BestMSR-VTT}
\end{table}

\clearpage
\newpage
% Negative example - MSVD - EtENet-GLN
\begin{table}[h!]
\begin{center}
\begin{tabular}{|l|p{6cm}|}
\hline
\multicolumn{2}{|c|}{EtENet-GLN} \\
\hline
Step 1 & {two girls are dancing} \\
Step 2 & {two girls are dancing} \\
References & \emph{a man dries off a woman}; 
\emph{couples were speaking}; 
\emph{a man is talking to a woman}; \\
\hline
Step 1 & {a dog is walking} \\
Step 2 & {a cat is walking} \\
References & \emph{a guinea pig chews on food}; 
\emph{the hamster is eating a carrot}; 
\emph{a rabbit is eating a carrot}; \\
\hline
Step 1 & {two men are playing} \\
Step 2 & {a man is riding a horse} \\
References & \emph{an elephant eats foliage}; 
\emph{the elephant is eating}; 
\emph{an elephant is eating grass}; \\
\hline
Step 1 & {a band is performing on a stage} \\
Step 2 & {a man is playing with a stage} \\
References & \emph{the flag is waving in the air}; 
\emph{the american flag flew in the wind}; 
\emph{the united states flag is waving}; \\
\hline
\multicolumn{2}{|c|}{EtENet-IRv2} \\
\hline
Step 1 & {a man is cutting a tomato} \\
Step 2 & {a man is cutting a tomato} \\
References & \emph{a man is putting a knife in a clamp};
\emph{a man is balancing a knife};
\emph{a man is keep the knife on the machine}; \\
\hline
Step 1 & {a group of people are playing} \\
Step 2 & {a baby is eating} \\
References & \emph{a woman puts stickers on her face};
\emph{the woman is putting stickers on their face};
\emph{a girl is addicting stricers}; \\
\hline
Step 1 & {two men are playing chess} \\
Step 2 & {a group of people are dancing} \\
References & \emph{a choir is singing};
\emph{the peoples are singing a song};
\emph{people are singing in church}; \\
\hline
Step 1 & {a cheetah is running} \\
Step 2 & {a lion is running} \\
References & \emph{a jackal is walking around in a field};
\emph{a jackal is running through grass};
\emph{predator running in a jungle}; \\
\hline
Step 1 & {a man is slicing a potato} \\
Step 2 & {a person is slicing a potato} \\
References & \emph{someone is using a juicer to squeeze the juice out of a lemon};
\emph{a man is preparing sweet lemon juice};
\emph{a man making orange juice}; \\
\hline
Step 1 & {a group of men are playing} \\
Step 2 & {a man is doing some sort of bread} \\
References & \emph{someone opens a pizza box containing pepperoni pizza};
\emph{a man opens a pizza box};
\emph{a person is opening a pizza box}; \\
\hline
\end{tabular}
\end{center}
\caption{Some negative examples on MSVD dataset}
\label{tab:NegExampleMSVD}
\end{table}

\newpage
% Negative example - MSR-VTT
\begin{table}[h!]
\begin{center}
\begin{tabular}{|l|p{6cm}|}
\hline
\multicolumn{2}{|c|}{EtENet-IRv2} \\
\hline
Step 1 & {a man is holding a gun} \\
Step 2 & {a man is holding a gun} \\
References & \emph{someone repairing or assembling a machine}; 
\emph{a man showing how to install grommets for a car engine}; 
\emph{a man is teaching how to use tools}; \\
\hline
Step 1 & {a man is playing a video game} \\
Step 2 & {a man is playing a video game} \\
References & \emph{a man is shooting a basketball ground};
\emph{a photographer describes the space he used for a photo shoot};
\emph{a photographer is taking photos}; \\
\hline
Step 1 & {a woman is singing} \\
Step 2 & {a woman is dancing} \\
References & \emph{a woman trying to escape in a television scene};
\emph{people are running on a sidewalk};
\emph{people running and a woman falls down}; \\
\hline
Step 1 & {a person is showing how to solve a toy} \\
Step 2 & {a person is showing how to solve a toy} \\
References & \emph{a person is working};
\emph{a man is teaching how to tie a fishing knot};
\emph{instructions for tying a knot}; \\
\hline
Step 1 & {a man is playing a video game} \\
Step 2 & {a man is talking to a man} \\
References & \emph{filming of action scenes in movie};
\emph{a man is filming a scene in the rain};
\emph{a video showing the making of the movie thor}; \\
\hline
Step 1 & {a cat is talking} \\
Step 2 & {a cat is talking to a cat} \\
References & \emph{a group of dogs are coming out of a container};
\emph{man whistles and a dozen puppies come running out of a small round box};
\emph{dogs are all sleeping together in a little room}; \\
\hline
Step 1 & {a man is talking about a car} \\
Step 2 & {a man is talking about a car} \\
References & \emph{video game scene of a guy looking at different cars};
\emph{cartoon play on the show};
\emph{a man playing video games}; \\
\hline
Step 1 & {a person is playing a video game} \\
Step 2 & {a man is talking about a car} \\
References & \emph{an animation presents something called project z};
\emph{someone is showing video graphic};
\emph{credits presented in 3d text}; \\
\hline
\end{tabular}
\end{center}
\caption{Some negative examples on MSR-VTT dataset}
\label{tab:NegExampleMSR-VTT}
\end{table}
